# Supplementary material for: Boosting End-to-End Database Isolation Checking via Mini-Transactions (Extended Version)
Source: arXiv:2504.02344 source file (2025-04-03)
Supplement: Supplementary file 1 [file abort-rate.tex]

% abort-rate.tex

%\section{Abort rate}
% \label{section:appendix-abort-rate}

%\begin{figure}
%	\centering
	%	\begin{minipage}[b]{0.3\textwidth}
		%		\centering
		%		\includegraphics[width = \textwidth]{figs/abortion-rate/ser-succ-keys.pdf}
		%		\caption{ser abortion rate comparison against \#txns/\#objects(8 sessions, 1000 txns, 20 ops/txn)}
		%		\label{fig:ser-abort-skew}
		%	\end{minipage}
	%	\begin{minipage}[b]{0.3\textwidth}
		%		\centering
		%		\includegraphics[width = \textwidth]{figs/abortion-rate/ser-succ-txns.pdf}
		%		\caption{ser abortion rate comparison against \#txns(8 sessions, 300 objects, 20 ops/txn)}
		%		\label{fig:ser-abort-txn}
		%	\end{minipage}
	%	\begin{minipage}[b]{0.49\columnwidth}
		%		\centering
%				\includegraphics[width = \columnwidth]{figs/abortion-rate/succ-sessions-intro.pdf}
%				\caption{The abortion rates
%						for executing GT and MT workloads (20 operations per transaction) in PostgreSQL.  %\#sessions(200 objects, 1000 txns, 20 ops/txn) 
%					}
%				\label{fig:ser-abort-session-intro}
		%	\end{minipage}

	%	\begin{minipage}[b]{0.3\textwidth}
		%		\centering
		%		\includegraphics[width = \textwidth]{figs/abortion-rate/si-succ-keys.pdf}
		%		\caption{si abortion rate comparison against \#txns/\#objects(8 sessions, 2000 txns, 20 ops/txn)}
		%		\label{fig:si-abort-skew}
		%	\end{minipage}
	%	\begin{minipage}[b]{0.3\textwidth}
		%		\centering
		%		\includegraphics[width = \textwidth]{figs/abortion-rate/si-succ-txns.pdf}
		%		\caption{si abortion rate comparison against \#txns(8 sessions, 500 objects, 20 ops/txn)}
		%		\label{fig:si-abort-txn}
		%	\end{minipage}
	%	\begin{minipage}[b]{0.3\textwidth}
		%		\centering
		%		\includegraphics[width = \textwidth]{figs/abortion-rate/si-succ-sessions.pdf}
		%		\caption{si abortion rate comparison against \#sessions(200 objects, 1000 txns, 20 ops/txn)}
		%		\label{fig:si-abort-session}
		%	\end{minipage}
	%\caption{examples of our empirical study}
	%\label{fig:motivation-bugs}
%\end{figure}
