# Supplementary material for: Boosting End-to-End Database Isolation Checking via Mini-Transactions (Extended Version)
Source: arXiv:2504.02344 source file (2025-04-03)
Supplement: Supplementary file 2 [file effectiveness.tex]

% effectiveness.tex

To evaluate the effectiveness of \ourtool in isoaltion checking,
we compare it against randomized testing of PostgreSQL 11.8
using general workloads, including list append and read-write registers,
with varying maximum transaction length of
2, 4, 6, 8, 10, and 12 operations.
Each run is required to successfully commit 3, 000 transactions.
We conduct 50 trials for each configuration
and report the average time for history generation and verification,
the average abort rate, and the number of bugs detected.
An ``exponential'' object-access distribution is used to
increase the likelihood of triggering bugs.

As shown in Figure~\ref{fig:bug-detection},
randomized testing with list append workloads
detects the highest number of bugs (49 out of 50 trials)
at a maximum transaction length of 8 operations.
At this length,
MTC (of maximum transaction length 4)
achieves approximately $2.0$ times faster
history generation and verification
compared to randomized testing with
both list append and read-write register workloads.
Additionally, MTC reduces the average abort rate
by about $28\%$ compared to randomized testing.
By detecting bugs in $14$ out of $50$ trials,
MTC demonstrates its effectiveness in identifying isolation anomalies.
