# Supplementary material for: Boosting End-to-End Database Isolation Checking via Mini-Transactions (Extended Version)
Source: arXiv:2504.02344 source file (2025-04-03)
Supplement: Supplementary file 3 [file si-validation-e2e.tex]

% si-validation-e2e.tex

% \begin{figure*}
% 	\centering
% 	\resizebox{.5\linewidth}{!}{
% 		\begin{tikzpicture}
% 			\centering
% 			\begin{axis}[
% 					hide axis,
% 					width=2cm, % Set width to minimum (1pt)
% 					height=2cm, % Set height to minimum (1pt)
% 					area legend,
% 					legend style={at={(1,-0.1)},anchor=south, legend columns=4,draw=none},
% 					/tikz/every even column/.append style={column sep=0.5cm}
% 				]
% 				\addlegendimage{color=red, pattern color=red, pattern=crosshatch}
% 				\addlegendentry{\footnotesize \ourtool gen}
% 				\addlegendimage{color=blue, pattern color=blue}
% 				\addlegendentry{\footnotesize PolySI gen}
% 				\addlegendimage{color=red, fill=red}
% 				\addlegendentry{\footnotesize \sitool}
% 				\addlegendimage{color=blue, pattern color=blue, pattern=crosshatch dots}
% 				\addlegendentry{\footnotesize PolySI}
% 				\addplot[draw=none] coordinates {(0,0)}; % Dummy plot for reference
% 			\end{axis}
% 		\end{tikzpicture}
% 	}

% 	\begin{subfigure}[b]{0.32\textwidth}
% 		\centering
% 		\includegraphics[width = \textwidth]{figs/comp-exp/si-e2e-txns.pdf}
% 	%	\caption{time against \#txns, e2e}
% 	\caption{}
% 		\label{fig:si-validation-e2e-txns}
% 	\end{subfigure}
% 		\hfill
% 	\begin{subfigure}[b]{0.32\textwidth}
% 		\centering
% 		\includegraphics[width = \textwidth]{figs/comp-exp/si-e2e-ops.pdf}
% 		%	\caption{time against \#ops, e2e}
% 		\caption{}
% 		\label{fig:si-validation-e2e-ops}
% 	\end{subfigure}
% 	\hfill
% 	\begin{subfigure}[b]{0.32\textwidth}
% 		\centering
% 		\includegraphics[width = \textwidth]{figs/comp-exp/si-e2e-keys.pdf}
% 	%	\caption{time against \#objects, e2e}
% 	\caption{}
% 		\label{fig:si-validation-e2e-keys}
% 	\end{subfigure}
% 	%	\hfill
% 	%	\begin{subfigure}[b]{0.2\textwidth}
% 	%	\centering
% 	%	\includegraphics[width = \textwidth]{figs/mm.jpeg}
% 	%	\caption{XX bug found in YY}
% 	%	\label{xx}
% 	%  \end{subfigure}
% 	\caption{End-to-end checking time for SI,
% 	  decomposed into history generation and verification.}
% 	\label{fig:si-validation-e2e}
% \end{figure*}
